# Supplementary material for: Stay Ahead of Poachers: Illegal Wildlife Poaching Prediction and Patrol Planning Under Uncertainty with Field Test Evaluations
Source: arXiv:1903.06669 source file (2019-11-06)
Supplement: Supplementary file 1 [file 9-Appendix.tex]

\appendix

\section{Runtime}

Algorithm runtime is shown in Table~\ref{table:runtime}, which averages among the three experiments we ran for each dataset. Overall, DTB-iW is the most efficient technique and runs nearly instantly. The SVB-iW model completes in under two minutes. However, GPB-iW is significantly more computationally expensive, requiring over 7~hours of computation on MFNP. All experiments were performed on 32-core machines with Intel 2.1~GHz processors and 264~GB of memory. 

%Note that computational efficiency is particularly important in this domain, because ranger stations are located in remote regions with extremely limited computing resources. We discovered that that we could dramatically improve runtime with GPB and GPB-iW with little to no trade-off in performance by using bagging classifiers on small subsets of the data. Without any bagging, runtime took over 126~hours in some cases. With greater bagging sampling on just 10--20\% of the data, we could reduce runtime to under 15~minutes. 

\begin{table}[h]
\centering
\caption{Average runtime (in sec) across each dataset}
\label{table:runtime}
\begin{tabular}{c|ccc}
\Xhline{2\arrayrulewidth}
& \textbf{MFNP} & \textbf{QENP} &\textbf{SWS} \\
\hline
\textbf{SVB} & 9.5 & 3.4 & 1.0 \\
\textbf{DTB} & 1.1 & 1.1 & 1.1 \\
\textbf{GPB} & 3887 & 1544 & 1.9 \\
\hline
\textbf{SVB-iW} & 67.3 & 24.1 & 3.1 \\
\textbf{DTB-iW} & 3.9 & 3.3 & 2.0 \\
\textbf{GPB-iW} & 27281 & 19211 & 121.1 \\
\Xhline{2\arrayrulewidth}
\end{tabular}
\end{table}

\vfill\null

\section{Performance}

To assess performance, we compute the standard machine learning metrics including AUC, precision, recall, and F1~score. We include the L\&L score, which is specifically designed for models learned on positive and unlabeled datasets~\cite{lee2003learning}. L\&L is defined as $\text{L\&L} = \frac{r^2}{\Pr[f(Te)=1]}$, where $r$ denotes recall and $\Pr[f(Te)=1]$ denotes the probability of a classifier~$f$ predicting a positive class label, estimated by the percentage of positive labels that a model predicts on a given test set. The maximum achievable L\&L score depends on the test set of interest, by setting $r = 1$ and using the percentage of positive labels in the test set for $\Pr[f(Te)=1]$. Thus, we also report the percentage of the maximum L\&L score obtained by each model: $\text{L\&L\%} = \frac{\text{L\&L}}{\max{\text{L\&L}}}$ (higher is better). Differing from past work, we also include the area under the precision-recall curve (PRC), which is considered a more informative metric for binary classification on imbalanced data~\cite{saito2015precision}.

Performance metrics for all three test sets on MFNP, QENP, and SWS are shown in Table~\ref{table:full_performance}.

\begin{table*}
\centering
\caption{Comparing performance of each model across all three datasets}
\label{table:full_performance}

\centerline{
\begin{tabular}{r|ccccccc|ccccccc|rrrrrrr}
\Xhline{2\arrayrulewidth}
 & \multicolumn{7}{c|}{\textbf{MFNP (2014)}} 
 & \multicolumn{7}{c|}{\textbf{MFNP (2015)}}
 & \multicolumn{7}{c}{\textbf{MFNP (2016)}}\\
& \textbf{AUC} & \textbf{PRC} & \textbf{Prec.} & \textbf{Rec.} & \textbf{F1} & \textbf{L\&L} & \textbf{L\&L\%} 
& \textbf{AUC} & \textbf{PRC} & \textbf{Prec.} & \textbf{Rec.} & \textbf{F1} & \textbf{L\&L} & \textbf{L\&L\%} 
& \textbf{AUC} & \textbf{PRC} &  \textbf{Prec.} & \textbf{Rec.} & \textbf{F1} & \textbf{L\&L} & \textbf{L\&L\%} \\
%& \textbf{AUC} & \textbf{Prec.} & \textbf{Rec.} & \textbf{F1} & \textbf{L\&L} & \textbf{L\&L\%} \\
 \hline
\textbf{SVB}
& 0.52 & 0.18 & 0.35 & 0.06 & 0.10 & 0.13 & 2.04 
& 0.51 & 0.13 & 0.17 & 0.03 & 0.06 & 0.04 & 0.56 
& 0.52 & 0.15 & 0.30 & 0.05 & 0.09 & 0.11 & 1.52
\\ \textbf{DTB}
& 0.59 & 0.22 & 0.20 & 0.62 & 0.30 & 0.76 & 12.38 
& 0.61 & 0.17 & 0.17 & 0.57 & 0.26 & 0.77 & 9.66 
& 0.60 & 0.20 & 0.16 & 0.74 & 0.26 & 0.89 & 11.87
\\ \textbf{GPB}
& 0.63 & 0.23 & 0.22 & 0.61 & 0.33 & 0.84 & 13.71 
& 0.66 & 0.20 & 0.19 & 0.65 & 0.30 & 1.00 & 12.55 
& 0.62 & 0.20 & 0.16 & 0.82 & 0.27 & 1.00 & 13.40
\\ \hline
\textbf{SVB-iW}
& 0.69 & 0.29 & 0.31 & 0.59 & 0.40 & 1.11 & 18.10 
& 0.68 & 0.26 & 0.31 & 0.40 & 0.35 & 0.99 & 12.36 
& 0.66 & 0.26 & 0.24 & 0.57 & 0.34 & 1.01 & 13.53
\\ \textbf{DTB-iW}
& 0.72 & 0.33 & 0.31 & 0.62 & 0.41 & 1.17 & 19.06 
& 0.71 & 0.30 & 0.32 & 0.39 & 0.35 & 0.98 & 12.28 
& 0.71 & 0.30 & 0.24 & 0.59 & 0.34 & 1.03 & 13.84
\\ \textbf{GPB-iW}
& 0.72 & 0.32 & 0.28 & 0.66 & 0.40 & 1.17 & 19.08 
& 0.71 & 0.28 & 0.33 & 0.35 & 0.34 & 0.92 & 11.58 
& 0.71 & 0.28 & 0.24 & 0.60 & 0.34 & 1.06 & 14.19
\\\Xhline{2\arrayrulewidth}
\end{tabular}
}

\bigskip

\centerline{
\begin{tabular}{r|ccccccc|ccccccc|rrrrrrr}
\Xhline{2\arrayrulewidth}
 & \multicolumn{7}{c|}{\textbf{QENP (2014)}} 
 & \multicolumn{7}{c|}{\textbf{QENP (2015)}}
 & \multicolumn{7}{c}{\textbf{QENP (2016)}}\\
& \textbf{AUC} & \textbf{PRC} & \textbf{Prec.} & \textbf{Rec.} & \textbf{F1} & \textbf{L\&L} & \textbf{L\&L\%} 
& \textbf{AUC} & \textbf{PRC} & \textbf{Prec.} & \textbf{Rec.} & \textbf{F1} & \textbf{L\&L} & \textbf{L\&L\%} 
& \textbf{AUC} & \textbf{PRC} &  \textbf{Prec.} & \textbf{Rec.} & \textbf{F1} & \textbf{L\&L} & \textbf{L\&L\%} \\
%& \textbf{AUC} & \textbf{Prec.} & \textbf{Rec.} & \textbf{F1} & \textbf{L\&L} & \textbf{L\&L\%} \\
 \hline
\textbf{SVB}
& 0.50 & 0.04 & 0.00 & 0.00 & 0.00 & 0.00 & 0.00 
& 0.50 & 0.06 & 0.00 & 0.00 & 0.00 & 0.00 & 0.00 
& 0.50 & 0.06 & 0.00 & 0.00 & 0.00 & 0.00 & 0.00
\\ \textbf{DTB}
& 0.68 & 0.08 & 0.10 & 0.40 & 0.16 & 1.11 & 4.12 
& 0.59 & 0.09 & 0.11 & 0.31 & 0.16 & 0.55 & 3.38 
& 0.63 & 0.10 & 0.12 & 0.35 & 0.18 & 0.76 & 4.28
\\ \textbf{GPC}	
& 0.69 & 0.10 & 0.08 & 0.35 & 0.13 & 0.78 & 2.88 
& 0.60 & 0.08 & 0.08 & 0.73 & 0.14 & 0.93 & 5.73 
& 0.60 & 0.09 & 0.09 & 0.44 & 0.15 & 0.69 & 3.90
\\ \hline
\textbf{SVB-iW}	
& 0.60 & 0.06 & 0.11 & 0.27 & 0.15 & 0.75 & 2.79 
& 0.62 & 0.14 & 0.18 & 0.30 & 0.23 & 0.89 & 5.48 
& 0.64 & 0.15 & 0.17 & 0.37 & 0.24 & 1.14 & 6.40
\\ \textbf{DTB-iW} 
& 0.72 & 0.09 & 0.12 & 0.27 & 0.17 & 0.87 & 3.22 
& 0.70 & 0.16 & 0.17 & 0.40 & 0.24 & 1.11 & 6.85 
& 0.74 & 0.20 & 0.24 & 0.32 & 0.27 & 1.36 & 7.67
\\ \textbf{GPC-iW}	
%% UPDATE WITH NEW RESULTS
& 0.64 & 0.07 & 0.11 & 0.15 & 0.13 & 0.44 & 1.61 
& 0.71 & 0.17 & 0.17 & 0.37 & 0.24 & 1.05 & 6.43 
& 0.74 & 0.20 & 0.23 & 0.24 & 0.24 & 1.01 & 5.66
\\\Xhline{2\arrayrulewidth}
\end{tabular}
}

\bigskip

\centerline{
\begin{tabular}{r|ccccccc|ccccccc|rrrrrrr}
\Xhline{2\arrayrulewidth}
 & \multicolumn{7}{c|}{\textbf{SWS (2016)}} 
 & \multicolumn{7}{c|}{\textbf{SWS (2017)}}
 & \multicolumn{7}{c}{\textbf{SWS (2018)}}\\
& \textbf{AUC} & \textbf{PRC} & \textbf{Prec.} & \textbf{Rec.} & \textbf{F1} & \textbf{L\&L} & \textbf{L\&L\%} 
& \textbf{AUC} & \textbf{PRC} & \textbf{Prec.} & \textbf{Rec.} & \textbf{F1} & \textbf{L\&L} & \textbf{L\&L\%} 
& \textbf{AUC} & \textbf{PRC} &  \textbf{Prec.} & \textbf{Rec.} & \textbf{F1} & \textbf{L\&L} & \textbf{L\&L\%} \\
%& \textbf{AUC} & \textbf{Prec.} & \textbf{Rec.} & \textbf{F1} & \textbf{L\&L} & \textbf{L\&L\%} \\
 \hline
\textbf{SVB}	
& 0.81 & 0.02 & 0.04 & 0.29 & 0.07 & 2.69 & 1.09 
& 0.68 & 0.00 & 0.01 & 0.09 & 0.02 & 0.61 & 0.08 
& 0.51 & 0.01 & 0.01 & 0.92 & 0.02 & 1.07 & 0.76
\\ \textbf{DTB}	
& 0.80 & 0.03 & 0.15 & 0.07 & 0.09 & 2.44 & 0.99 
& 0.71 & 0.00 & 0.01 & 0.09 & 0.01 & 0.44 & 0.06 
& 0.53 & 0.01 & 0.01 & 0.05 & 0.02 & 0.10 & 0.07
\\ \textbf{GPC}	
& 0.78 & 0.04 & 0.29 & 0.07 & 0.11 & 4.54 & 1.84 
& 0.73 & 0.01 & 0.01 & 0.18 & 0.02 & 1.35 & 0.17 
& 0.55 & 0.01 & 0.02 & 0.03 & 0.02 & 0.08 & 0.05
\\ \hline
\textbf{SVB-iW}	
& 0.76 & 0.01 & 0.03 & 0.19 & 0.05 & 1.21 & 0.49 
& 0.86 & 0.01 & 0.06 & 0.09 & 0.07 & 3.90 & 0.51 
& 0.67 & 0.01 & 0.02 & 0.30 & 0.03 & 0.72 & 0.51
\\ \textbf{DTB-iW} 
& 0.72 & 0.02 & 0.03 & 0.19 & 0.05 & 1.44 & 0.58 
& 0.83 & 0.01 & 0.03 & 0.09 & 0.04 & 1.80 & 0.23 
& 0.69 & 0.01 & 0.01 & 0.43 & 0.03 & 0.81 & 0.60
\\ \textbf{GPC-iW}	
%% UPDATE WITH NEW RESULTS
& 0.68 & 0.01 & 0.02 & 0.10 & 0.03 & 0.35 & 0.14 
& 0.82 & 0.01 & 0.03 & 0.09 & 0.05 & 2.19 & 0.28 
& 0.71 & 0.01 & 0.02 & 0.73 & 0.03 & 1.52 & 1.07
\\\Xhline{2\arrayrulewidth}
\end{tabular}
}

\end{table*}
